# Supplementary material for: U-Mind: A Unified Framework for Real-Time Multimodal Interaction with Audiovisual Generation
Source: arXiv:2602.23739 source file (2026-02-27)
Supplement: Supplementary file 1 [file 6_suppl.tex]

% \clearpage
\setcounter{page}{1}
% \maketitlesupplementary
\begin{figure*}
    \centering
    \includegraphics[width = \textwidth]{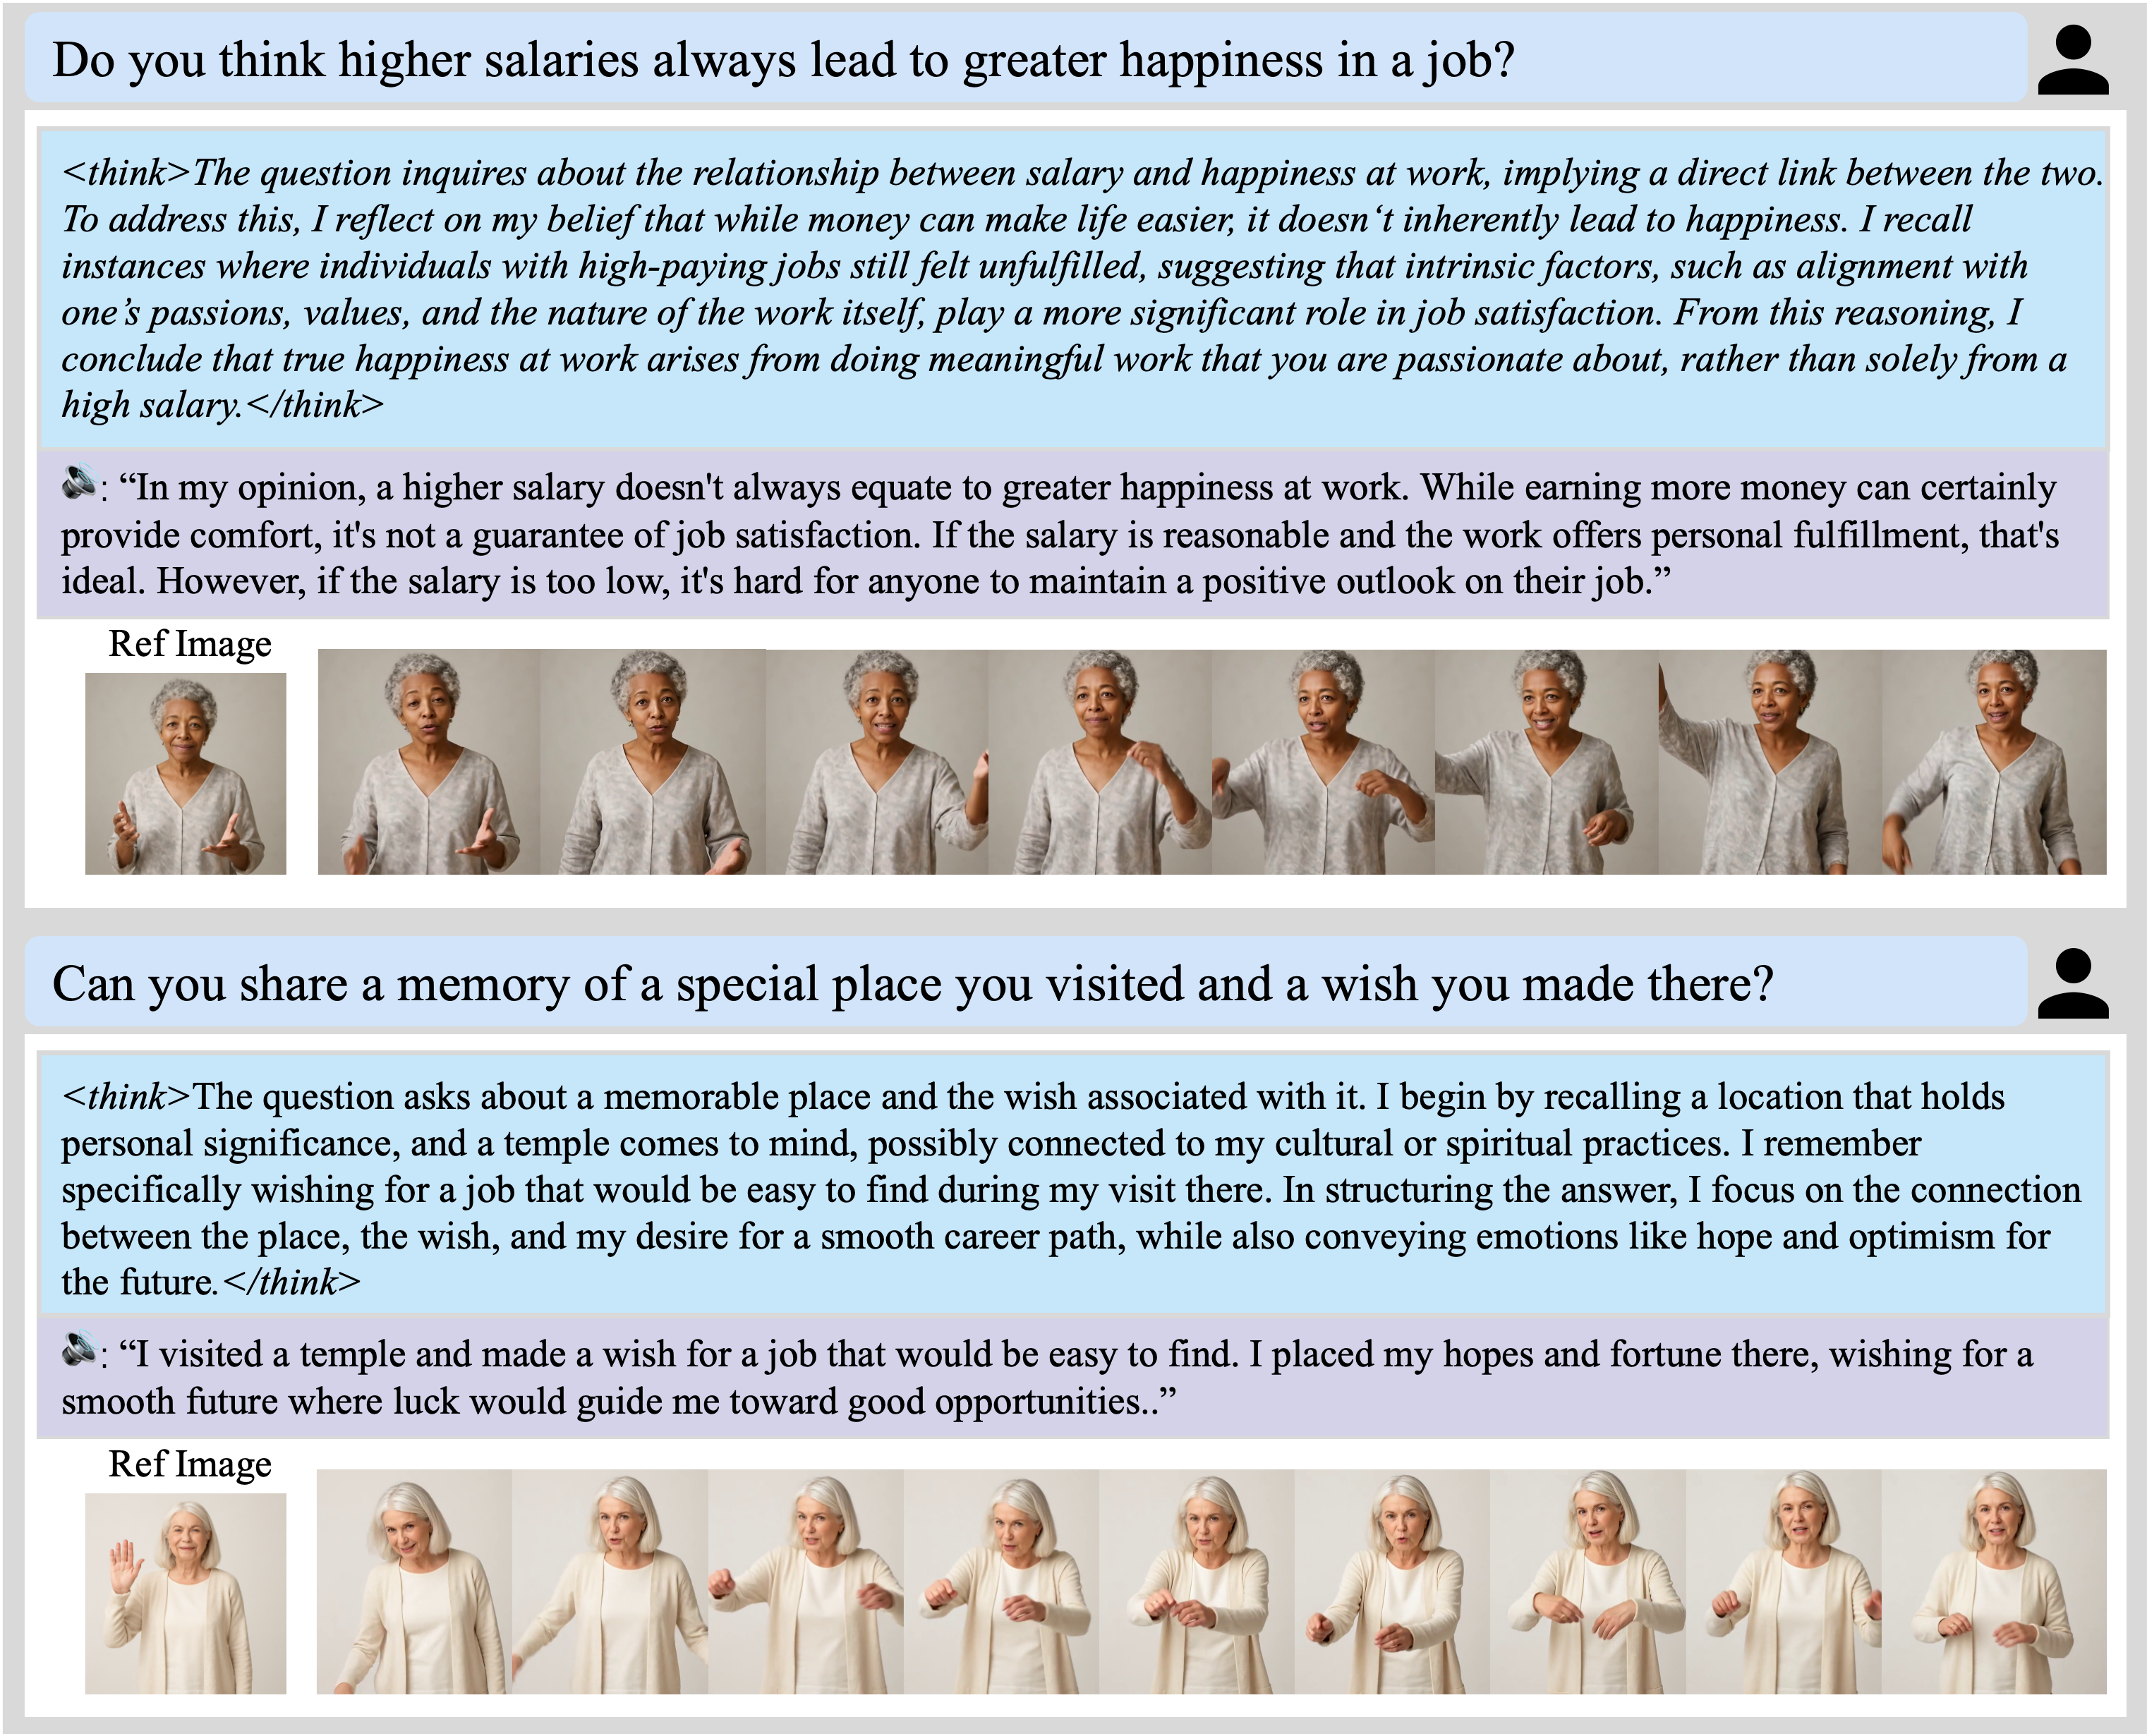}
    \caption{More Multimodal Dialogue Results.}
    \label{fig:dialogue_results_sup}
\end{figure*}
% , instruction following, and 3D-consistent generation
To provide a more complete understanding of our proposed U-Mind system, this supplementary material presents (1) detailed descriptions of our data construction pipeline, including reasoning-augmented annotations and multimodal synthesis preparation; (2) expanded implementation details, covering model architecture, tokenizer training, and experimental setup; and (3) additional qualitative results that illustrate its strengths in multimodal dialogue. These materials aim to clarify key design choices and support the reproducibility of our work.

\section{Data Construction Details}

To support the training of U-Mind across dialogue, instruction-following, and full-stack video generation, we construct a comprehensive multimodal dataset that integrates both benchmark resources and proprietary corpora. The data pipeline is organized into two primary components: core datasets for multimodal alignment and reasoning, and auxiliary corpora for supporting text2speech (TTS) and video rendering.

\subsection{Multimodal Training Datasets}

% \textbf{Dialogue and S2M Supervision.}
\noindent\textbf{Multimodal Dialogue Supervision.} We build a reasoning-enhanced dialogue dataset based on BEAT v2~\cite{liu2024emage}, which provides paired speech and motion data. For each utterance or gesture segment, we prompt a large language model (Qwen3) to generate three question--answer--reasoning triplets, injecting explicit CoT-style traces into the original corpus. The generated textual answers are then converted to audio using a high-quality neural TTS system (Orpheus-TTS~\cite{orpheus2025}), resulting in coherent multimodal dialogue samples. For original speech recordings, we apply Whisper~\cite{whisper2022} to obtain accurate transcriptions. This pipeline yields a dataset containing 10k reasoning-enhanced S2M examples and over 30k multimodal QA--reasoning pairs, enabling symbolic and physical grounding in dialogue settings.

\noindent\textbf{Instruction-Following Supervision.}
We construct a CoT-augmented instruction-following dataset based on HumanML3D~\cite{Guo_2022_CVPR}, which provides natural language descriptions paired with 3D motion data. For each description, we prompt a large language model (Qwen3) to generate three question–answer–reasoning triplets, enabling hierarchical task decomposition and intermediate planning. This process yields 16k high-quality T2M samples, each enriched with explicit symbolic reasoning signals.
To convert symbolic supervision into multimodal alignment targets, all Qwen3-generated responses are synthesized into speech using Orpheus-TTS~\cite{orpheus2025}, forming synchronized text–speech–motion triples.
% Additionally, raw audio in the HumanML3D dataset is transcribed via Whisper~\cite{whisper2022}, ensuring consistent textual supervision for grounding motion generation.
% \textbf{Instruction-Following and T2M Supervision.}
\subsection{Auxiliary Corpora for Speech and Video Modules}

% \textbf{Conversational Reasoning and TTS.}
\noindent\textbf{Conversational Reasoning and TTS.}
To further enhance symbolic planning and speech generation capabilities, we incorporate two external datasets: OpenOrca \cite{mukherjee2023orca}, a high-quality open-domain corpus rich in multi-turn conversational reasoning, and Common Voice \cite{ardila2020common}, a multilingual crowd-sourced speech dataset that improves the TTS model’s prosody, phonemic diversity, and naturalness. By mixing these resources into our training pipeline, the model benefits from both abstract reasoning supervision and diverse acoustic grounding, leading to more fluent, expressive, and semantically coherent multimodal outputs.

% \textbf{Video Renderer Training.}
\noindent\textbf{Video Renderer Training.}
To enable photorealistic and temporally aligned video generation, we adopt two complementary rendering pipelines. First, we collect a 500-hour proprietary human video corpus annotated with 2D keypoints using DWPose~\cite{yang2023effective}, which is used to train a diffusion-based renderer based on the WAN~\cite{wan2025wan} backbone. Second, we train a Gaussian Splatting renderer on the TaoAvatar~\cite{chen2025taoavatar} dataset, utilizing 3D SMPL-X annotations to enable direct pose-driven 3D video synthesis. These two renderers provide complementary views: while diffusion models produce high-fidelity 2D renderings from 2D pose inputs, Gaussian-based renderers directly generate consistent 3D avatar videos from SMPL-X poses, supporting diverse real-time generation scenarios.
These components together support U-Mind’s full-stack, instruction-following multimodal interaction capabilities.

\section{Additional Implementation Details}

This section provides implementation details for the tokenizer modules, model configuration, training strategy, and inference settings used in the U-Mind system.

\subsection{Motion Tokenizer} We employ a residual VQ-VAE architecture~\cite{zhang2024semantic, siyaoduolando} to discretize 3D motion sequences into compact token representations. Specifically, we use a 4-layer residual quantization scheme with a temporal downsampling ratio of 4. To enhance numerical stability and preserve geometric continuity, each input sequence of SMPL-X parameters is first converted into a 6D continuous pose representation before encoding.
These continuous poses are then encoded into discrete codebook indices, enabling token-level modeling of motion. This design ensures a balance between fidelity and compression, facilitating efficient multimodal learning.
% \begin{figure*}
%     \centering
%     \includegraphics[width = \textwidth]{img/A4.jpg}
%     \caption{More Instruct Following Results.}
%     \label{fig:instruct_results_sup}
% \end{figure*}
\subsection{Speech Tokenizer}
For speech representation, we utilize the SpeechTokenizer \cite{zhang2023speechtokenizer} module to discretize waveform audio into acoustic tokens. This tokenizer captures phonetic and prosodic information suitable for both speech synthesis and alignment. During multimodal training, the speech encoder, like all modality encoders, is kept frozen to preserve stable representations and avoid catastrophic forgetting.

\subsection{Model Backbone and Token Prediction}
Our multimodal language model is based on the LLaMA2-7B \cite{touvron2023llama} architecture, initialized with the pretrained weights from AnyGPT \cite{zhan2024anygpt}. We extend the tokenizer's codebook to include motion and speech tokens and train the model using a unified next-token prediction objective. Given a prompt sequence, the model autoregressively generates text, acoustic, and motion tokens in a unified token stream.

% \begin{figure*}
%     \centering
%     \includegraphics[width = \textwidth]{img/A4.jpg}
%     \caption{3D Consistency Results.}
%     \label{fig:3D_results_sup}
% \end{figure*}
\subsection{Training Details}
\noindent\textbf{Motion Tokenizer.}
The motion tokenizer is trained using a 4-layer residual VQ-VAE architecture with a temporal downsampling ratio of 4. To ensure robust learning and smooth quantization, SMPL-X pose parameters are first converted into 6D continuous representations. The tokenizer is optimized using the AdamW optimizer with a learning rate of 1e-5, $\beta$ values of [0.9, 0.999], and no weight decay. We apply a learning rate scheduler with milestones at epochs 50, 150, and 250, decaying the learning rate by a factor of 0.4 at each milestone. Exponential moving average (EMA) with a momentum of 0.99 is employed to stabilize training. The model is trained with a batch size of 256 on 8 H100 GPUs.

\noindent\textbf{U-Mind Backbond.}
We adopt a two-stage training pipeline to balance perceptual grounding with instruction alignment. In the 	pre-training stage, we use a learning rate of 1e-4, a batch size of 4, a maximum sequence length of 2048, and a cosine learning rate scheduler. Training is conducted on 8 H100 GPUs using bfloat16 precision. In the instruction tuning stage, we continue training from the pre-trained checkpoint with a reduced learning rate of 2e-5, keeping the batch size and sequence length unchanged. This staged approach allows the model to first acquire modality fluency without catastrophic forgetting, and then align with high-level interactive behaviors under a stabilized training regime.

Each input prompt is formatted with modality-aware delimiters. The model outputs a \texttt{<think>} block for symbolic reasoning before generating perceptual modalities. Modal tokens are aligned in a consistent autoregressive order to preserve temporal coherence and facilitate video rendering.
We initialize text encoders from LLaMA2-7B, and retain the pretrained SpeechTokenizer and motion VQ-VAE modules as frozen during all LLM training. This modular design ensures representational stability while leveraging large-scale pretrained knowledge.

\noindent\textbf{Diffusion-based Renderer.}
Our diffusion-based video renderer is built upon the WAN~\cite{wan2025wan} backbone. To enable fine-grained control over multimodal synthesis, we introduce cross-attention layers into the video decoder that inject motion and audio features, allowing the model to produce synchronized body movement and speech directly from the autoregressively generated token sequence.

We train the model on 25fps video clips using 16×H100 GPUs with the following settings: a constant learning rate of $1\mathrm{e}{-5}$ with 100 warm-up steps, Adam optimizer with weight decay of 0.01, gradient clipping at 1.0, and bfloat16 mixed-precision training. We adopt optical flow-based filtering during preprocessing, using a minimum flow threshold of 0 and filtering frames based on percentile scores capped at 5. This ensures temporal coherence and training stability during synthesis learning.

\noindent\textbf{Gaussian-based Renderer.}
Our Gaussian-based renderer is developed following the pipelines of \cite{zhan2025real, chen2025taoavatar}, leveraging 3D point cloud accumulation and SMPL-X-driven body control. The model is trained using a learning rate of $5\mathrm{e}{-4}$ with a cosine annealing scheduler, Adam optimizer with a weight decay of 0.01, and runs on a single H100 GPU. 
% This renderer enables efficient and high-fidelity 3D synthesis with low latency, making it suitable for real-time interaction scenarios.

\subsection{Inference Settings}
During inference, the model operates in an autoregressive decoding mode with a unified token stream. The prompt first triggers internal \texttt{<think>} reasoning, followed by text, speech, and motion token generation. Generated acoustic tokens are converted to waveforms and re-encoded for video synthesis, while motion tokens are decoded into SMPL-X poses. Video rendering is subsequently performed by either a diffusion-based or Gaussian-based renderer, depending on the output mode.

% \subsection{Tokenizer and Prompt Formatting}
% Each input prompt is formatted with modality-aware delimiters. The model outputs a \texttt{<think>} block for symbolic reasoning before generating perceptual modalities. Modal tokens are aligned in a consistent autoregressive order to preserve temporal coherence and facilitate video rendering.

% \subsection{Pretrained Modules}
% We initialize text encoders from LLaMA2-7B, and retain the pretrained SpeechTokenizer and motion VQ-VAE modules as frozen during all LLM training. This modular design ensures representational stability while leveraging large-scale pretrained knowledge.

\subsection{Experimental Settings and Baselines}

\noindent\textbf{Data Splits.}
For all experiments, we adopt a 7:1 train-test split for each dataset. Multimodal dialogue and instruction-following evaluations are conducted on our curated test sets built from BEAT v2 and HumanML3D, respectively. For foundational tasks such as text-to-motion (T2M) and speech-to-motion (S2M), we use the similar test sets from HumanML3D~\cite{Guo_2022_CVPR} and BEAT v2~\cite{liu2024emage}.

\noindent\textbf{Baselines and Training Protocol.}
We compare against several representative baselines introduced in the main paper. For SOLAMI~\cite{jiang2025solami}, since pretrained weights are not publicly released, we train the model from scratch on our dataset using the official implementation and training protocol. For all other baselines, including LOM~\cite{chen2025language}, EMAGE~\cite{liu2024emage}, CaMN~\cite{liu2022beat}, and DisCo~\cite{liu2022disco}, we use their publicly released weights and codebases for fair comparison.
To benchmark performance of a cascaded pipeline, we also construct a baseline system composed of LLaMA2-Chat-7B~\cite{touvron2023llama} for dialogue, Orpheus-TTS~\cite{orpheus2025} for speech synthesis, and LOM\cite{chen2025language} for motion generation, simulating a non-unified approach to multimodal interaction.

\section{Additional Qualitative Results}

% To further illustrate the capabilities of our system, we present additional qualitative results across three representative categories: (1) multimodal dialogue understanding, (2) instruction-following, and (3) 3D vsualization consistency.

% \noindent\textbf{More Multimodal Dialogue Examples.}
% \subsection{More Multimodal Dialogue Examples.}
We provide extra cases in Fig \ref{fig:dialogue_results_sup} that demonstrate the model's ability to interpret diverse user queries, perform intermediate reasoning, and generate coherent multimodal responses. These examples cover open-domain and context-dependent questions, showing how the system grounds its answers with appropriate gestures, synchronized speech, and internally reasoning traces. The responses reflect both semantic understanding and communicative clarity.

% \noindent\textbf{More Instruction-Following Examples.}
% \subsection{More Instruction-Following Examples.}
% We showcase complex instruction-following scenarios where the model is prompted to execute specific tasks with precise spatiotemporal coordination. Each case involves a prompt, an internal planning segment, and the resulting multimodal outputs. Our model consistently demonstrates strong intent alignment, accurate sequencing, and expressive multimodal behavior across a variety of verbal and non-verbal commands.

% % \noindent\textbf{3D-Consistent Rendering Examples.}
% \subsection{3D-Consistent Rendering Examples.}
% We present videos rendered from multiple viewpoints to demonstrate the 3D consistency of U-Mind's generated motion. These examples are rendered from the same SMPL-X pose sequences but viewed from different camera angles, verifying that our generated motions are spatially coherent and semantically consistent under rotation. As shown in the video supplement, gestures remain stable and expressive, and the body movements maintain continuity and realism across changing perspectives.
